# Supplementary material for: Improving Black-box Robustness with In-Context Rewriting
Source: arXiv:2402.08225 source file (2024-08-05)
Supplement: Supplementary file 1 [file Correlations.tex]

\subsection{Entropy Correltations Details}

In Section \ref{selective-aug}, we study whether the entropy of the original prediction's class probability disitrubution is predictive of whether TTA will change the model's prediction. This is of interest since avoiding potentially expensive augmentations imprives the method's effecuency. Below are the p-values for the point biserial corelations.
