# Supplementary material for: Improving Black-box Robustness with In-Context Rewriting
Source: arXiv:2402.08225 source file (2024-08-05)
Supplement: Supplementary file 2 [file Limitations.tex]

\subsection{Limitations}

\paragraph{Exhaustiveness.} Test-time augmentation's flexibility comes with its ability to be leveraged on a wide range of tasks, models, and augmentation policies. As such, our work presents a partial evaluation of TTA's effectiveness. We opted to focus on a set of representative short-form text classification tasks---a common setting for evaluating NLP techniques. There may be tasks, datasets, or augmentation methods where TTA performs better than in our setting of study. 

\paragraph{Frontier Models.} Our work focuses on relatively small models, with Falcon-7b being the largest task model we study. These results do not give conclusive evidence of whether TTA is robustly effective for the largest currently available models, such as GPT-4, Claude, and Bard. However, that we demonstrate TTA generally becoming less effective across model scales gives some evidence that TTA is unlikely to be robustly useful in the settings we studied for these largest models.
